# Supplementary material for: Decoupling DNS Update Timing from TTL Values
Source: arXiv:2409.10207 source file (2024-09-16)
Supplement: Supplementary file 1 [file wheelappendix.tex]

%\appendix

\newpage

% \gal{I removed the related work from the appendix.}
% \gal{I kept the wheel appendix pretty much the same as it were,
% except for the modular case that I copied from the thesis}
%\section{APPENDIX: Related Work}
%\label{app-related}
%%%%%%%%%%%%%%%%%%%%%%%%%%
%Our model is based on, and inspired by, a long history of theoretical
%models in distributed computing. To gain some perspective, we offer
%here a brief review.
%% More details are provided in
%% \sectionref{sec-related}.
%
%
%Historically, distributed computing is split along the dichotomy of
%message passing vs shared memory~\cite{Pierre10}. While message
%passing is deemed the ``right'' model for network algorithms, the
%shared memory model is the abstraction of choice for programming
%multi-core machines. 
%
%The prominent theoretical message-passing models are LOCAL~\cite{L92},
%and its derived CONGEST~\cite{Peleg:book}. In these models, a system
%is represented by a connected (typically undirected) graph, in which
%nodes represent processors and edges represent communication links.
%The basic actions are message send (initiated by processors) and
%message receive (initiated by links). Local computation is assumed to
%be unbounded and instantaneous, so that the running time of a network
%algorithm is just the number of communication rounds it requires.
%%
%In the LOCAL model, message size is unbounded, and therefore the only
%restriction for a node to retrieve any piece of information  is
%the number of hops separating the node from the location of that
%information.
%% As a consequence,  a statement
%% of the form ``node $v$ can output after $t$ rounds'' means that the output at
%% node $v$ is independent of any input (value or action) located more
%% than $t$ hops away from $v$ \cite{L92}. This property makes LOCAL
%% a clean model to analyze locality in graph problems.
%%
%The CONGEST model is a refined version of LOCAL, with the additional
%restriction that messages may be only $O(\log n)$-bits long, where $n$ is the number of
%nodes.%
%\footnote{%
%  More precisely, the number of bits in a message is a parameter of
%  the CONGEST model, and the default value of that parameter is
%  $O(\log n)$.  This value is chosen for reasons similar to the choice
%  of word size in the sequential RAM model~\cite{AhoHU74}: this way, a
%  message can contain a constant number of references to nodes and
%  edges, and possibly other
%  variables whose magnitude is bounded by a polynomial in $n$.
%%
%}
%Thus, CONGEST % is traditionally
%% thought of as more realistic than LOCAL, as it
%accounts not only for the
%distance information has to traverse, but also for information volume  
%and  the
%bandwidth available for its transportation.
%
%% It is important to note that in the absence of faults, both network
%% algorithms models can be assumed synchronous: If processors and links
%% are reliable but run in different speeds, one can use a
%% synchronizer~\cite{A-85} to hide these differing speeds, allowing
%% algorithms to be developed in the synchronous model (in which
%% processors advance in lockstep rounds, where each round consists of
%% receive-compute-send substeps).
%While most algorithms in the LOCAL and CONGEST models assume
%fault-free (and hence synchronous) executions, in the distributed
%shared memory model, asynchrony and faults are the primary source of
%difficulty. Usually, in the shared memory model one assumes that there
%is a collection of ``registers,'' accessible by multiple threads of
%computation that run at different speeds and may suffer crash or even
%Byzantine faults (see, e.g., \cite{AttiyaW}). The main issues in this
%model are coordination and fault-tolerance. Typically, the only
%quantitative hint to communication cost is the number and size of the
%shared registers.
%
%%%%%%%%%
%\ignore{
%  Quite a few papers consider the combination of message
%passing and shared memory, e.g., 
%\cite{MNV,logp-new,qsm,BSP,AdlerGMR-99}.
%The uniqueness of the \CWC model with respect to past work is that it  combines passive storage nodes with a  message passing network with restrictions on the links bandwidth.
%}
%
%%%%%%%%%%%%%%%%%%%%%%%%
%An early attempt to somehow
%restrict bandwidth in parallel computation, albeit indirectly, is due
%to Mansour et al.~\cite{MNV}, who considered PRAM with $m$ words of
%shared memory, $p$ processors and input length $n$, in the regime
%where $m\ll p\ll n$. The LogP model~\cite{logp-new} by Culler et al.\
%aimed at adjusting the PRAM model to network-based realizations.
%Another proposal that models shared memory
%explicitly is the QSM model of Gibbons et al.~\cite{qsm}, in which
%there is an explicit (typically uniform)  limit on the bandwidth
%connecting processors to shared memory. QSM is 
%similar to our \CWC model, except that there is no network connecting
%processors directly. A thorough comparison of bandwidth limitations in
%variants of the BSP model~\cite{BSP} and of QSM is presented by Adler et
%al.~\cite{AdlerGMR-99}.  We note that LogP and BSP do not
%provide  shared memory as a primitive object: the idea is to describe
%systems in a way that allows implementations of abstract shared memory.
%%%%%%%%%%%%%%%%%%%%%%%%%%%%%%%%%%%%%%
%
%Another proposal that combines message passing with shared memory
%is
%the ``m\&m'' model, recently proposed by Aguilera et
%al.~\cite{ABCGPT18}. The m\&m
%model assumes that processes can exchange messages via
%a fully connected network, and there are shared registers as well,
%where each shared register is accessible only by a subset of the 
%processes.
%The focus in~\cite{ABCGPT18} is on solvability of distributed tasks in 
%the 
%presence of
%failures, rather than performance.
%
%Recently, with the advent of massive data centers and high-bandwidth
%communication, new variants were proposed to facilitate  a formal study
%of algorithms in these environments. 
%%We mention here two.  
%The CONGESTED CLIQUE (CC) model~\cite{LotkerPPP-05}
%is a special case of CONGEST,
%where the underlying communication graph is assumed to be fully
%connected (i.e., a clique over the processors). % In this model, all
%% information is reachable within 1 hop---but it can be retrieved only
%% in quanta of $O(\log)$ bits. Theoretically, one can view  CC as an
%% orthogonal model to LOCAL: whereas in LOCAL the only constraint is
%% length (distance), in CC the only constraint is width (congestion).
%% Practically, i
%The CC model is appropriate for computing \emph{in} the cloud, as it
%% Even though the model was originally conceived for theoretical study, 
%% it 
%has been shown that under some relatively mild
%conditions, algorithms designed for the CC 
%model can be implemented in the MapReduce model, i.e., run in 
%datacenters~\cite{HegemanP-15}. Another model for computing in the
%cloud is the MPC model~\cite{KSV10}. 
%%
%% Thus it appears that the long-accepted model of communication modeled
%% by graph is losing prominence in the message passing world, even
%% though the actual underlying hardware works by message passing.
%Very recently, the HYBRID model~\cite{AHKSS20} was proposed as a 
%combination of CC
%with classical graph-based communication. % The HYBRID
%% marries the LOCAL and the CC models as follows. T
%More specifically, the HYBRID model assumes the existence of  two
%communication networks: one for local communication between neighbors,
%where links are typically of infinite bandwidth (exactly like LOCAL);
%the other network is a \emph{node-congested} clique, i.e., a node can
%communicate with every other node directly via ``global links,'' but
%there is a small upper bound (typically $O(\log n)$) on 
%the total number 
%of messages a node can
%send or receive via these global links in a round.
%Even though the model was presented only recently, there is already 
%a line of algorithmic work in it, in particular for computing
%shortest paths~\cite{AHKSS20,KS-20,CLP20}.
%% (we stress again that the
%%capacity restriction does not apply
%%to the local links).
%
%%%%%  %%%%%
%\textbf{Discussion.} Intuitively, our  \CWC model can be viewed as
%the classical 
%CONGEST model over the processors, augmented by
%special cloud nodes  (object stores)
%connected to some (typically, many) compute nodes.
%To reflect modern demands and availability of resources, we relax the 
%very stringent bandwidth 
%allowance of
%CONGEST, and usually envision networks with much larger link
%bandwidth (e.g., $n^\epsilon$ for some $\epsilon>0$).
%
%Considering previous network models, it appears that  HYBRID  is
%the closest to  \CWC, even though HYBRID
%was not expressly designed to model the cloud. In our view,
%\CWC is indeed more 
%appropriate for computation with  the cloud. First, % it appears that 
%in most
%cases, global communication (modeled by clique edges in HYBRID) is 
%limited by link bandwidth, unlike 
%HYBRID's
%node capacity constraint, which seems somewhat artificial. Second, HYBRID is 
%not readily amenable to  model multiple clouds, while this is a
%natural property of \CWC . 
%%Third,
%%the focus in the HYBRID model papers \cite{AHKSS20,KS-20} is on graph
%%topology problems, which appear less useful, in some sense, in the
%%presence of global communication such as a clique of a cloud, since
%%global links distort topology in a deep sense.
%
%Regarding shared memory models, we are unaware of topology-based
%bandwidth restriction on shared memory access in distributed
%models. In some general-purpose parallel computation models (based on 
%BSP~\cite{BSP}), communication capabilities are specified using a 
%few
%global parameters such as latency and throughput%  (see
%% \sectionref{sec-related})
%, but these models deliberately abstract topology away.
%% (with the exception of \cite{MNV}, see
%% \ref{sec-related}).
%In distributed (asynchronous) shared memory, the number of bits 
%that need to be
%transferred to and from the shared memory is seldom explicitly
%analyzed. 
%%Our modeling of explicit communication with the shared
%%storage may therefore be useful even without local
%%communication links.
%
%
%%\todo{Mention dynamic flow. We can copy / rely on
%%	my intro in \sectionref{ssec:dynamic-flow}}


\section{APPENDIX: Non-Commutative Operators and the Wheel Settings}
\label{sec:wheel-appendix}
%%%%%%%%%%%%%%%%%%%%%%%%%%%%%

In this section we elaborate on the cases and theorems discussed in
\sectionref{sec:wheel}.

\ignore{

In this section we consider \CCW for
non-commutative operators such as Matrix Multiplication.

First note that \algref{alg:ccw-hi} and \theoremref{thm-ccw-covers-ub} from
\sectionref{ssec:combining}
may still apply, as long as the ordering of the nodes matches
one of the possible ordering that is achieved by the algorithm.
% For example, if there is a cover $\cC$ of the system
% such that in each cluster all nodes are consecutive,
% and such that the combination of all nodes in the cluster is achievable
% in $O(\Zmax(C))$ rounds without using cloud links,
% the upper bound of \theoremref{thm-ccw-covers-ub}
% would still apply, as long as the order
% between the clusters is one that can be preserved by \algref{alg:ccw-high:overlap}
% (i.e., all clusters of a single color class are consecutive).
% Otherwise, an upper bound of $O(\Zmax(C) \cdot \load(C) \cdot \log |C|)$
% can be achieved by \algref{alg:ccw-hi} by discarding
% the use of \algref{alg:ccw-high:overlap}, and instead using \algref{alg:ccw-high:node}
% on all subsets $C_l$ in parallel, using multiplexing.
However, it is not always likely that the inputs are located according
to the ordering of some (unspecified) cover. Instead, we believe that
in the case of a non-commutative combining operator, it is reasonable
to assume that processing nodes are physically connected 
according to their combining order. Closing the cycle for symmetry and
adding a cloud link from each processor, we arrive at the wheel
topology, which we study in this section.


% We therefore consider in this section a system with the
% wheel-topology: processors numbered $0$ through $n-1$ 
% that contain only this cycle and the targeted cloud node.
% \todo{in the intro, make the part about the wheel network a definition, and then
% reference it here}
% Unlike \sectionref{ssec:combining}, in this section due to the topology assumptions,
% we do not require the graph to be locally wide.

Our main result in this section is an algorithm for \CCW for arbitrary
wheel topology that works in time which is a logarithmic factor larger
than optimal. In contrast to the result of \theoremref{thm-ccw-ub} that
applied only to graphs with fat links, here we analyze the wheel
topology with arbitrary bandwidths.
% $O(Z_{\max}\log n)$ rounds in the wheel settings, where $Z_{\max}$ is the maximal timespan
% of cloud intervals (cf.\ \defref{def:intervals2} and \theoremref{thm-aw-ub}).
We note that by using
standard methods \cite{LadnerF-80}, the algorithm presented in this section can be extended to
compute, with the same asymptotic time complexity, all prefix sums,
i.e., compute, for each $0\le j<n$, $\bigotimes_{i=0}^jS_i$.

We distinguish between \emph{holistic} and
\emph{modular} combining operators, defined as follows.
In modular combining, one can apply the combining
operator to aligned, equal-length parts of operands to get the output
corresponding to that part. For example, this is the case with vector
(or matrix) addition: to compute any entry in the sum, all that is
needed is the corresponding entries in the summands.
If the operand is not modular, it is called holistic
(e.g., matrix multiplication).
% no part of the product can be computed without both operands being
% % the product can be computed only when both operands are
% known in the entirety.
% This is the case, for example, with matrix
% multiplication.  
We show that in the modular case, using pipelining, a logarithmic
factor can be shaved off the running time (more precisely, converted
into an additive term), as can be seen in \theoremref{thm-aw-modular}.

% In \sectionref{ssec:wheel-holistic},
% we start by reducing the definitions of cloud clusters and of cluster's timespan
% to the wheel setting,
% as well as adjust the algorithms and theorems of \sectionref{ssec:combining},
% to provide an upper bound of $\Zmax \log n$ to \CCW.
% In \sectionref{ssec:wheel-modular}, we explain how to speed up the algorithm
% in the case of modular combining.
}

We start by defining the cloud intervals of nodes in the wheel settings.
For completeness of exposition we repeat \defref{def-intervals}  here:
\para{
{\bf \defref{def-intervals}:}
The \textbf{cloud bandwidth} of a processing node $i \in V_p$ in a
	given wheel graph is
    $\bc(i)\DEF w(i,v_c)$.
	An \textbf{interval}
	$\interval{i}{i\tp k}\DEF\Set{i,i\tp 1,\ldots,i\tp k}\subseteq V$ is a path
	of processing nodes in the ring. Given an interval $I=[i,i+k]$,  $|I|=k+1$ is its \textbf{size}, and $k$ is its
	\textbf{length}.  The \textbf{cloud bandwidth} of $I$,
	denoted $\bc(I)$, is the sum of the cloud bandwidth of all nodes in
	$I$: $\bc(I)=\sum_{i\in I}\bc(i)$.  The \textbf{bottleneck
		bandwidth} of $I$, denoted $\blmin(I)$, is the smallest bandwidth
	of a link in the interval:
	$\blmin(I)=\min\Set{w(i,i\tp1)\mid i,i\tp1\in I}$.  If  $|I|=1$, define $\blmin(I) = \infty$.
}
\ignore{%%%%
See \defref{def-intervals} for the complete definitions of intervals and their parameters.
% We start with the concept of intervals that refines the concept of
% clusters (\defref{def-clusters}) to the case of the wheel topology.
In short, for an interval $I=[i,i+k]$, the cloud bandwidth of $I$ is
$\bc(I)=\sum_{i\in I}\bc(i)$
and the bottleneck bandwidth of $I$ is
$\blmin(I)=\min\Set{w(i,i\tp1)\mid i,i\tp1\in I}$.  If  $|I|=1$, we define $\blmin(I) = \infty$.
}%%%%%%%%

For ease of presentation we consider the ``one sided'' case in which
node $i$ does not use one of its incident ring links.  As we shall
see, this limitation does not increase the time complexity by more
than a constant factor. Hence we consider the case in which node $i$
cannot send messages on its counterclockwise link.

% We start by defining the concepts of intervals, which are the clusters
% parallels in the wheel settings.

% Since we no longer assume that the graph is locally wide,
% narrow bandwidth on the local links may limit the
% reachability of cloud bandwidth of remote nodes, in addition to their distance.
% Fortunately, in the
% wheel topology, we can easily find the sweet spot that balances the
% constraints optimally (up to a constant factor).
% We therefore update the definitions regarding cloud-clusters (\defref{def-Bi}).

\begin{definition}\label{def-Ii}
	Let $i$ be a processing node in the wheel settings. We define the following quantities for
	clockwise intervals; counterclockwise intervals are defined
	analogously. 
	\begin{compactitem}
		\item \label{def:kc}
		$\kCR{i}$ is the length
		of the smallest interval starting at $i$, for which the product of
		its size by the total bandwidth to the cloud along the interval
		exceeds $s$,  i.e.,
		$$\kCR{i} = \min
          \left(\Set{n}\,\cup\, \Set{k\mid \left(k\tp 1\right) \cdot \bc([i,i\tp k]) \ge
			s} \right)~.
          $$
% 		$\kCR{i}=\min\Set{k\mid \left(k\tp 1\right) \cdot \bc([i,i\tp k]) \ge
% 			s}$. $\kCR{i}=n$ if no such integer exists.
		\item \label{def:kl}
		$\kLR{i}$ is the length
		of the smallest clockwise interval starting at node $i$, for which the bandwidth
		of the clockwise-boundary link bandwidth is smaller than the total
		cloud bandwidth of the interval, i.e.,
		$$\kLR{i} = \min
          \left(\Set{n}\,\cup\, \Set{k\mid w(i\tp k,i\tp k\tp 1)<\bc(\interval{i}{i\tp k})} \right)~.
          $$
% 		$\kLR{i}=\min\Set{k\mid w(i\tp k,i\tp k\tp 1)<\bc(\interval{i}{i\tp k})}$,
% 		or $n$ if no such integer exists.
		\item $\kR{i}= \min\Set{\kCR{i}, \kLR{i}}$.
		\item $\IR{i} = \interval{i}{i\tp \kR{i}} $. The interval $\IR{i}$ is
		called the (clockwise) \textbf{cloud interval} of node $i$.
		\item $\ZR{i} = |\IR{i}| + \dfrac{s}{\blmin(\IR{i})} +
		\dfrac{s}{\bc(\IR{i})}$. $\ZR{i}$ is the \textbf{timespan} of the
		(clockwise) cloud interval of $i$.
	\end{compactitem}
\end{definition}
% Note that $\kR{i}$ is easily computable.
% We start by analyzing the time complexity of \CW using intervals.







\subsection{\CW and \CR}

\begin{theorem}\label{theorem:CW_UB_interval}
	Given the cloud interval $I_i$ of node $i$,
	\algref{alg:cw-hi} solves the $s$-bits $\CW_i$ problem in $O(\ZR{i})$ rounds.
\end{theorem}
\Proof
The BFS tree of the interval would be a simple line graph, that is the whole interval.
Note that Step \ref{cw-alg-send-local} requires
$O\left(|\IR{i}| + {\frac{s}{\bLminR{i}}} \right)$ rounds: there are
$s$ bits to send over $\Theta(|I_i|)$ hops with bottleneck bandwidth $\phi(I_i)$.
The rest of the time analysis is the same as in \theoremref{theorem:CW_UB}.
\QED

We have the following immediate consequence.
%\begin{theorem}\label{theorem:CW_UB_wheel}
%	\algref{alg:cw-hi} solves the $s$-bits $\CW_i$ problem in $O(\ZR{i})$ rounds
%	on $\IR{i}$.
%\end{theorem}

\begin{theorem}\label{theorem:two_sided_UB}
	Let $Z_i^\ell$ and $Z_i^r$ denote the timespans of the counterclockwise and the clockwise cloud intervals of $i$, respectively. Then $\CW_i$ can be solved in $O(\min(Z_i^\ell,Z_i^r))$ rounds.
	%	There is an algorithm that writes an $s$-bits message originating
	%	from node $i$ to the cloud, that requires at most $O(\ZR{i})$
	%	rounds.
\end{theorem}


We now turn to the lower bound.
% same as we did in \sectionref{single-lb} we assume that
% the $s$-bits string $S$ that node $i$ needs to write is incompressible.
% Similarly to our upper bound strategy, we first prove the lower bound
% for ``one-sided'' intervals, and then extend it to the general case.

\begin{theorem}
	\label{theorem:one_sided_LB}
	In the wheel settings, any algorithm for $\CW_i$
	which does not use link $({i\tm 1}, i)$ requires $\Omega(\ZR{i})$ rounds.
\end{theorem}
\Proof
We show that each term
of $\ZR{i}$ is a lower bound on the running time of any algorithm
solving $\CW_i$.
%
% The theorem follows from \lemmaref{lemma:interval_length}, \lemmaref{lemma:interval_BN} and \lemmaref{lemma-phi}.
% \QED

% Similarly to \corollaryref{cor-ub}, we have the following corollary
% for the uniform wheel.
% \begin{corollary}\label{cor-lb}
% 	In the uniform wheel topology with cloud bandwidth $\bc$ and local
% 	link bandwidth $\bl$, any algorithm for \CW requires at least
% 	$\Omega\left({s\over\bl}+\min(\sqrt{s\over\bc},{\bl\over\bc})\right)$
% 	rounds if $\bl\ge\bc$, and $\Omega({s\over\bc})$ otherwise.
% \end{corollary}
%
%
% \begin{lemma}
%	\label{lemma:interval_length}
First, note that any algorithm for $\CW_i$
	that does not use edge $({i\tm 1}, i)$ requires 
	$\Omega(\kCR{i}) \ge \Omega \left( \kR{i}\right) = \Omega \left( |\IR{i}|\right)$
	rounds,
% \end{lemma}
% \Proof
due to the exact same arguments as in \lemmaref{lemma:cluster_diameter}.
% we can get a lower bound of $\kCR{i}$.
% The lemma is completed by noting that $\kR{i} \le \kCR{i}$ by definition.
%
%Let $A$ be an algorithm for $\CW_i$
%that does not use link $({i\tm 1}, i)$ and runs in $t_A$ rounds.
%If $t_A \ge n$ then $t_A \ge \kR{i}$ and we are done. Otherwise,
%we count the number of bits of $S$ that can get to the cloud in $t_A$
%rounds.
%Since $S$ is initially stored in $i$, and since link $({i\tm 1},
%i)$ is not used, 
%in round $t$  only the nodes in
%$\interval{i}{i\tp t\tm1}$ can write to the cloud
%parts of $S$.
%It follows that in a given round $t$,
%at most $\bc([i,i\tp t\tm1])$ bits of
%information are sent to the cloud and therefore, overall $A$
%writes to the cloud at most
%$\sum_{t=1}^{t_A}\bc([i,i\tp t\tm1]) \le t_A\cdot\bc([i,i\tp t_A\tm1])$
%bits. Hence, by assumption that  $A$ solves $\CW_i$,
%we must have $t_A\cdot\bc([i,i\tp t_A\tm1]) \ge s$. Since by definition,
%$\kCR{i}$ is the minimal 
%integer%
%\footnote{
%	$\kCR{i}$ may be $n$ if no such integer exists, but $t_A$ is an integer
%	that satisfies the $\kCR{i}$ formula so this is not the case.
%}
%$\ell$ such that
%$(\ell \tp 1)\sum_{j=i}^{i+\ell} \bC{j} \ge s$, we get that
%$t_A \tm 1 \ge \kCR{i} \ge \kR{i}$ and the lemma follows. \QED
%
%
%\begin{lemma}
%	\label{lemma:interval_BN}

Next, we claim that	any algorithm for $\CW_i$
	which does not use edge $({i\tm 1}, i)$ requires 
	$\Omega({s}/{\blmin(\IR{i})})$ rounds.
% \end{lemma}
% \Proof
        To see that note first that if $\kR{i}=0$, then
        $\blmin(\IR{i})=\infty$ and the claim is trivial.  Otherwise,
        let $(j,j\tp 1)\in E$ be any link in $\IR{i}$ with
        $\bL{j}{j\tp 1} = \bLminR{i}$.  Note that $j-i<\kR{i}$ because
        $j+1\in I_i$.  Consider the total bandwidth of links emanating
        from the interval $I' \DEF \interval{i}{j} $. Since we assume
        that the link $(i\tm1,i)$ is not used, the number of bits that
        can leave $I'$ in $t$ rounds is at most
        $t\cdot\left(\bc(I')+ \bL{j}{j\tp 1}\right)$.  Notice
        that % $s$ bits of the file originate at node $i$ and are written
% to the cloud, and thus
at least $s$ bits have to leave $I'$.
%
Observe that $\bc(I') \le \bL{j}{j\tp 1}$, because otherwise we would have
$\kLR{i}=j-i$, contradicting the fact that $k(i)>j-i$.
Therefore, any
algorithm $A$ that solves $\CW_i$ in $t_A$ rounds satisfies
$$
s~\le~t_A\cdot\left(\bc(I') + \bL{j}{j\tp 1} \right)
~\le~ 2t_A\cdot \bL{j}{j\tp 1}
~=~ 2t_A\cdot \bLminR{i} ~,
$$
and the claim follows.

Finally, we claim that
%\begin{lemma}\label{lemma-phi}
any algorithm $A$ for $\CW_i$ which does not use edge $({i\tm 1}, i)$
requires $\Omega \left({s}/{\bC{\IR{i}}} \right)$ rounds.
%\end{lemma}
%
%\Proof Let $A$ be any algorithm that solves $\CW_i$ in $t_A$ rounds.
To see that, recall that $\kR{i} = \min(\kCR{i}, \kLR{i})$.  If
$\kR{i}=n$ then $\IR{i}$ contains all processor nodes $V_p$, and the
claim is obvious, as no more than $\bC{V_p}$ bits can be written to
the cloud in a single round.  Otherwise, we consider the two cases: If
$\kR{i} = \kCR{i}$, then $\kR{i} \ge {s}/{\bC{\IR{i}}} - 1$ by
definition, and we are done since $t_A = \Omega(\kR{i})$.
% by \lemmaref{lemma:interval_length}.
Otherwise, $\kR{i} = \kLR{i}$. Let
us denote $w_R=\bL{i\tp \kR{i}}{i\tp \kR{i}\tp1}$. In this case we
have $w_R < \bc(\IR{i})$.  We count how many bits can leave $\IR{i}$.
% Similarly to \lemmaref{lemma:interval_BN},
In a single round, at most
$\bC{\IR{i}}$ bits can leave through the cloud links, and at most
$w_R$ bits can leave through the local links. Since $A$ solves
$\CW_i$, we must have
$ s ~\le~t_A\cdot\left(\bC{\IR{i}} +w_R\right) ~\le~ 2t_A \cdot
\bC{\IR{i}} ~,$ and hence
$t_A = \Omega\left({s}/{\bC{\IR{i}}} \right)$.  \QED


\begin{theorem}\label{theorem:two_sided_LB}
	Let $Z_i^\ell$ and $Z_i^r$ denote the timespans of the counterclockwise and the clockwise cloud intervals of $i$, respectively. Then $\CW_i$ requires
	$\Omega(\min(Z_i^\ell,Z_i^r))$ rounds in the wheel settings.
	%	There is an algorithm that writes an $s$-bits message originating
	%	from node $i$ to the cloud, that requires at most $O(\ZR{i})$
	%	rounds.
\end{theorem}
\Proof
Let $T$ be the minimum time required to perform $\CW_i$.
Due to \lemmaref{lem:schedule-iff-dynamic}, % and \theoremref{thm-cw},
we know that there is a dynamic flow mapping with
time horizon $T$ and flow value $s$ from node $i$ to the cloud.
Let $f$ be such a mapping.
We assume that no flow is transferred \emph{to} the source node $i$, as we can modify $f$
so that these flow units would not be sent from $i$ at all until the point
where they were previously sent back to $i$.
Let $s_L$ and $s_R$ be the total amount of flow that is transferred on links
$(i-1,i)$ and $(i,i+1)$, respectively, and
assume \WLOG that $s_R \ge s_L$.
Let $f'$ be a new dynamic flow mapping which is the same as $f$, except that no
flow is transferred on link $(i-1,i)$.
Since $f$ is a valid dynamic flow that transfers all $s$ flow units from $i$ to the cloud,
$f'$ has flow value at least $s-s_L$.
Let $A$ be a schedule derived from $f'$. The runtime of $A$ is at most $T$ rounds.
Let $A'$ be a schedule that runs $A$ twice: $A'$ would transfer $2(s-s_L)$ bits from node $i$
to the cloud. Since $s \ge s_R+s_L$, we get that:
$2(s-s_L) = 2s -2s_L \ge s + s_L + s_R -2s_L \ge s$, and thus $A'$ solves $\CW_i$
without using link $(i-1,i)$.
From \theoremref{theorem:one_sided_LB}, we get a lower bound for $2T$ of
$\Omega(Z_i^r) = \Omega(\min(Z_i^\ell,Z_i^r))$.
\QED


From \theoremref{theorem:two_sided_UB} and \theoremref{theorem:two_sided_LB}
we get the following corollary for the uniform wheel:
\begin{corollary}\label{cor-ub}
	In the uniform wheel topology with cloud bandwidth $\bc$ and local
	link bandwidth $\bl\ge\bc$, \CW can be solved in
	$\Theta\left({s\over\bl}+\min(\sqrt{s\over\bc},{\bl\over\bc})\right)$
	rounds. If $\bl<\bc$, the running time is $\Theta(s/\bc)$ rounds.
\end{corollary}
\Proof
If $\bl<\bc$, $\kLR{i}=0$, $\phi(I_i)=\infty$ and the result follows.
Otherwise, by definition we have $\kCR{i}=\sqrt{s/\bc}-1$ and
$\kLR{i}=\bl/\bc-1$, hence $|\IR{i}|=O(\min(\sqrt{s/\bc},\bl/\bc))$. It
follows that $\bc(\IR{i})=O(\min(\sqrt{s\cdot bc},\bl))$. The result follows by
noting that
$\bLminR{i}=\bl$.
\QED
\noindent
For example, for $\bc=\sqrt{s}$ and $\bl\ge s^{3/4}$, the
running time is $O(s^{1/4})$.


\emph{Remark.}
    Notice that the same upper and lower bounds hold for the $\CR_i$ problem as well.
%\end{remark}



% \todo{Prove the lower bound for both directions using flow arguments.}

% \todo{Add the same upper and lower bounds for \CR}

\subsection{Holistic Combining}
\label{ssec:wheel-holistic}


We are now ready to adapt \theoremref{thm-ccw-covers-ub}
to the wheel settings.
%For that matter we define $\Zmax$ similarly to \defref{graph-Zmax}:
%$\Zmax = \max_{i\in V_p} \ZR{i}$. 

\begin{definition}\label{def:intervals2}
  Given an $n$-node wheel, let $\IR{i}$ be the cloud interval of $i$
  with the smaller timespan (cf.\ \defref{def-Ii}).  Define
  $j_{\max} = \argmax_i\Set{|\IR{i}|}$,
  $j_c = \argmin_i \Set{\bC{\IR{i}}}$, and
  $j_\ell = \argmin_i \Set{\bLminR{i}}$.  Finally, define
  $Z_{\max} = {|\IR{j_{\max}}| + \frac{s}{\bLminR{j_\ell}} +
    \frac{s}{\bC{\IR{j_c}}} }$.
\end{definition}
In words: $j_{\max}$ is the node with the longest cloud interval,
$j_c$ is the node whose cloud interval has the least cloud bandwidth, and
$j_\ell$ is the node whose cloud interval has the narrowest bottleneck.


Let $C$ be the set of all cloud intervals $\IR{i}$.
\begin{theorem}\label{thm-ccw-intervals-ub:appendix}
	In the wheel settings,
	\CCW can be solved in
	$O(\Zmax \log n)$ rounds
	by \algref{alg:ccw-hi}
\end{theorem}

%\boaz{no coloring in sec.4}
The main difference that we can use to our advantage between the wheel case and
the general case, is that in the wheel case,
for any minimal cover $C'$, $\load(C') \le 2$ (see \lemmaref{lem-coverload}).
We can therefore use the cover $C$ to build a minimal cover $C'$,
and then have the multiplexing of \algref{alg:ccw-hi} add only a constant factor
to the runtime.
%only $3$ color classes in the run of \algref{alg:ccw-hi}.

We do that by adding another preprocessing stage to \algref{alg:ccw-hi},
in which we
select a cover $C' \subseteq C$ such that every
node is a member of either one or two intervals of $C'$.  It is
straightforward to find such a cover, say, by a greedy
algorithm. Concretely, a cover with a minimal \emph{number of intervals} is
found by the algorithm in \cite{min-circle-cover} (in $O(n\log n)$
sequential time). The covers produced by \cite{min-circle-cover}  are sufficient
for that matter, as the following lemma states.
\begin{lemma}
	\label{lem-coverload}
	Let $C$ be a collection of intervals and denote
	$U=\bigcup_{I\in C}I$.  Let $C'\subseteq C$
	be a minimal-cardinality cover of $U$, and let $\load_{C'}(i)=
	|\{I\in C' : I\ni i\}|$. Then for all
	$i\in U$, $1\le \load_{C'}(i)\le 2$.
\end{lemma}
\Proof Clearly $\load_{C'}(i)\ge1$ for all $i\in U$ since $C'$ is
a cover of $U$. For the upper bound, first note that by
the minimality of $|C'|$, there are no intervals $I,I'\in
C'$ such that $I\subseteq I'$,  because in this case $I$ could have
been discarded. This implies that the right-endpoints of intervals in $C'$
are all distinct, as well as the left-endpoints.
Now, assume for 
contradiction, that there exist three intervals
$I,I',I''\in C'$ such that $I\cap I'\cap I''\ne\emptyset$
(i.e., there is at least one node which is a member of all three).
Then $I\cup I'\cup I''$ is a contiguous interval.
Let $l=\min(I\cup I'\cup I'')$ and $r=\max(I\cup I'\cup I'')$.%
\footnote{
	The notation $\max(I)$ for an interval $I$ refers to the
	clockwise-end node of the interval.
}
By counting, one of the three intervals, say  $I$,
has no endpoint in $\Set{l,r}$. But this means
that $I\subseteq I'\cup I''$, i.e., 
we can discard $I$, in contradiction to the minimality of $|C'|$.
\QED

%\begin{corollary}\label{cor-intersect}
%	Any interval in $C'$ intersects at most two other intervals in $C'$,
%	i.e., $\load(C')=2$.
%\end{corollary}
%
%Therefore, according to \corollaryref{cor-intersect}, $C'$ can be partitioned into $3$
%color classes such that all intervals in a single color class are pairwise disjoint.


As for the ``low levels'' of the algorithm, i.e. Steps \ref{ccw-startloop}--\ref{ccw-endloop},
a little different approach is required instead of running \algref{alg:ccw-low},
due to the limited local bandwidth.
We present the time analysis for these steps with the following lemma:


\begin{lemma}\label{lem-lo}
	Steps \ref{ccw-startloop}--\ref{ccw-endloop}
	of \algref{alg:ccw-hi} terminate in
	$O\left(|I_{j_{\max}}|+\log|I_{j_{\max}}|\cdot{s\over\phi(I_{j_\ell})}\right)$
	rounds in the wheel settings, with $P_I$ stored in the rightmost node of $I$ for each
	interval $I\in C'$. 
\end{lemma}
\Proof
First, we require
that each input $S_i$ is associated with a single
interval in $C'$. To this end, we use the rule that if a node $i$ is a member
in two intervals 
$I$ and $I'$,
then its input $S_i$ is associated with the interval $I$ satisfying
$\max(I)<\max(I')$, and a unit input $\Unit$ is associated with $i$ in
the context of $I'$, where $\Unit$ is  the unit (neutral) operand for
$\otimes$.
Intuitively, this rule means that the overlapping regions in an
interval are associated with the ``left'' (counterclockwise) interval.

Second, we assume that the interval size, and therefore the number
of leaves in its computation tree, is a power of $2$. Otherwise, let
$p=2^{\ceil{\log|I|}}$ (i.e., $p$ is $|I|$ rounded 
up to the next power of $2$). When doing tree computation over an interval
$I$, we extend it (virtually) to a complete binary tree with $p$
leaves, where the leftmost $p-|I|$ leaves have the unit input
$\Unit$. These leaves are emulated by the leftmost node of $I$ (the
emulation is trivial).

Assume now that we wish to compute the combined value of an interval
$I$ whose length is a power of $2$.
Let $S_i^j$ denote the product of $S_i,\ldots,S_j$.
Computation of the combined value
of interval $I$ whose length is a power of $2$ proceeds in {stages},
where each stage $\ell$ computes all level-$\ell$ products in
parallel.  The algorithm maintains the invariant that after $S_i^j$ is
computed, it is stored in node $j$ (by definition, for all
$0\le i< n$, $S_i^i$ is initially stored at node $i$).  The
computation of a stage is performed as follows.

Let $S_i^{j}=S_i^k\otimes S_{k+1}^j$ be a product we wish to compute
at level $\ell$, and let $S_i^k, S_{k+1}^j$ be the values held by its
children. Note that $k+1-i=j-k=2^{\ell-1}$.  The algorithm forwards
$S_{i}^k$ from node ${k}$ to node $j$, which multiplies it by (the
locally stored) $S_{k+1}^j$, thus computing $S_i^j$, which is stored
in node $j$ for the next level. This way, the number of communication
rounds is just the time required to forward $s$ bits from ${k}$ to
$j$. Using pipelining, this is done in
$j-k+{s\over\phi([k,j])}=2^{\ell-1}+{s\over\phi([k,j])} \le
2^{\ell-1}+{s\over\phi(I)}$
rounds,
%\footnote{\interval{k}{j} is contained within some cloud interval,
%	therefore its bottleneck can not exceed $\phi(I_{j_\ell})$.}
and hence the total time required to compute the product
of all inputs of any interval $I$ is at most
\begin{equation}
	\label{eq:aw4}
	\sum_{\ell=1}^{\ceil{\log|I|}}\left(2^{\ell-1}+{s\over\phi(I)} \right)
	~\le~ 2\left(|I|+\log|I|\cdot{s\over\phi(I)}\right)~.
\end{equation}

Now back to the proof of \lemmaref{lem-lo}.
%\begin{lemma}\label{lem-lo}
%	Steps \ref{aw-colors}--\ref{aw-endloop} % \ref{aw-4}
%	of the algorithm terminate in
%	$O\left(|I_{j_{\max}}|+\log|I_{j_{\max}}|\cdot{s\over\phi(I_{j_\ell})}\right)$
%	rounds, with $P_I$ stored in the rightmost node of $I$ for each
%	interval $I\in C$. 
%\end{lemma}
%\Proof
Correctness is obvious. As for the complexity analysis:
%consider iteration $l$ of the loop of Step
%\ref{ccw-colors}. In this iteration, only intervals from $C_l$ apply in
%line \ref{ccw-local}, and since they are disjoint, their executions are
%independent.
By \Eqr{eq:aw4},   every interval $B\in C$ completes line
\ref{ccw-local} in
% $I$ from , we have by \defref{def:intervals2}
% that all intervals in $C_l$, and hence iteration $l$, complete in
at most
$O\left(|I_{j_{\max}}|+\log|I_{j_{\max}}|\cdot{s\over\phi(I_{j_\ell})}\right)$
rounds.
Multiplying this bound by $\load(C)\le 2$ due to the multiplexing,
%Summing this bound over $l=1,2,3$,
we conclude that the loop of
line \ref{ccw-startloop} completes after
$O\left(|I_{j_{\max}}|+\log|I_{j_{\max}}|\cdot{s\over\phi(I_{j_\ell})}\right)$
rounds.
\QED


\begin{lemma}\label{lem-hi}
	In the wheel settings,
	Step \ref{ccw-high} of \algref{alg:ccw-hi}
	terminates in
	$O(\Zmax \cdot \log n)$
	rounds.
\end{lemma}
\Proof
The usage of \algref{alg:ccw-high:node} remains as it were in the fat-links case.
By \lemmaref{ccw-lem-hi}, Step \ref{ccw-high} requires 
$O(\Zmax(C') \cdot \load(C') \cdot \log |C'|)$ rounds.
Noting that $|C'|\le |C| \le n$ and that all intervals in $C'$ are cloud intervals,
we get an upper bound of
$O(\Zmax \cdot 2 \cdot \log n) = O(\Zmax \cdot \log n)$ rounds.
\QED

The proof of \theoremref{thm-ccw-intervals-ub:appendix}
is completed as follows.
%by noting that in \algref{alg:ccw-hi},
%there is no need for \algref{alg:ccw-high:overlap}.
%Since the overlap entails only a constant blowup in the runtime,
%there is no need to reduce the problem to a case of a single color class,
%but instead \algref{alg:ccw-high:node} can be ran on all $3$ color classes
%simultaneously, by using multiplexing.
The correctness of the algorithm is derived from the general case
(\theoremref{thm-ccw-covers-ub}). As for the time analysis:
The ``low levels'' of the algorithm (Steps \ref{ccw-startloop}--\ref{ccw-endloop})
require $O(\Zmax \log n)$ according to \lemmaref{lem-lo},
noting that $|I_{j_{\max}}|\le n$ and 
that  $Z_{\max} = {|\IR{j_{\max}}| + \frac{s}{\bLminR{j_\ell}} +
\frac{s}{\bC{\IR{j_c}}} }$ by definition.
The ``high level'' of the algorithm (Step \ref{ccw-high})
requires $O(\Zmax \cdot \log{n})$ according to \lemmaref{lem-hi}.

All in all, the algorithm terminates in $O(\Zmax \cdot \log{n})$ rounds.
\QED


\para{Remark: Interval containing node $0$.}  In the case that
$\otimes$ is not commutative, the cover $C'$ may need
to be patched: In this case, we require that
the interval that contains node $0$ does not contain node $n-1$.
If this is not the case after computing the cover, let $I \in C'$ be an interval
that contains both. Partition $I$ 
into two subintervals $I=I_L \cup I_R$, where $I_L$ is the part that ends with
node $n-1$, and 
$I_R$ is the part that starts with node $0$. $I_L$ and $I_R$ replace
$I$ in the cover $C'$ for all purposes, except work: any work assigned
to either 
$I_L$ or $I_R$ will be executed by all nodes of $I$. This may incur an
additional constant slowdown due to multiplexing.


We finish with the lower bound.

\begin{theorem}\label{thm-aw-lb}
	Any algorithm for \CCW in the wheel topology requires 
	$\Omega(Z_{\max})$
	rounds. 
\end{theorem}

\Proof Same as in \theoremref{theorem:CCW-LB}, $\Omega(Z_i)$ is a
lower bound for every node $i$, by reduction from $\CW_i$.
Recall that
$\ZR{i} = {|\IR{i}| + {{s}\over{\bLminR{i}}} + {{s}\over{\bC{\IR{i}}}}}$.
For index $j_{\max}$ we get a lower bound of
$\Omega(Z_{j_{\max}}) \in \Omega(|\IR{j_{\max}}|)$.
For index $j_\ell$ we get a lower bound of
$\Omega(Z_{j_N}) \in \Omega({{s}/{\bLminR{j_\ell}}})$.
For index $j_c$ we get a lower bound of
$\Omega(Z_{j_C}) \in \Omega\left( {s}/{\bC{\IR{j_c}} }\right)$.
%
Summing them all up, gives the desired lower bound. \QED


\emph{Remark.}
    We note that similar upper and lower bounds of $O(\Zmax)$ and $\Omega(\Zmax)$ hold
    for the \CCR problem, similarly to the proofs in \sectionref{sec:CCR}.
% \end{remark}



\subsection{Modular Combining}
\label{ssec:wheel-modular}

%\smallskip\noindent
%Finally, we distinguish between \emph{holistic} and
%\emph{modular} combining operators, defined as follows.
%In modular combining, one can apply the combining
%operator to aligned, equal-length parts of operands to get the output
%corresponding to that part. For example, this is the case with vector
%(or matrix) addition: to compute any entry in the sum, all that is
%needed is the corresponding entries in the summands.
%If the operand is not modular, it is called holistic
%(e.g., matrix multiplication).
%% no part of the product can be computed without both operands being
%% % the product can be computed only when both operands are
%% known in the entirety.
%% This is the case, for example, with matrix
%% multiplication.  
%We call the aligned parts of the operands \emph{grains}, and their maximal size
%$g$ is the \emph{grain size}.
%See \defref{def:modular-op} for the full definition.
%We show that in the modular case, using pipelining, a logarithmic
%factor can be shaved off the running time (more precisely, converted
%into an additive term), as can be seen in the following theorem:
%
%
%\begin{theorem}[See \theoremref{thm-aw-modular:appendix}]\label{thm-aw-modular}
%Let
%	$j_{\max} = \argmax_i\Set{|\IR{i}|}$,
%	$j_c = \argmin_i \Set{\bC{\IR{i}}}$,
%	$j_\ell = \argmin_i \Set{\bLminR{i}}$, and
%	$Z_{\max} = {|\IR{j_{\max}}| + {s}/{\bLminR{j_\ell}} + s/{\bC{\IR{j_c}}} }$.
%	Suppose  $\otimes$ is modular with
%	grain size $g$. Then \CCW can be solved in
%	$O\left(Z_{\max}
%	+|I_{j_{\max}}|\ceil{\frac{g}{\phi(I_{j_{\ell}})}}
%	+\ceil{\frac{g}{\bC{\IR{j_c}}}}\log n\right)$.
%\end{theorem}



Intuitively, an operator is a modular combining operator if it can
be applied to aligned pieces of the operands and obtain the
corresponding piece of the result. For example, bit-wise operations
are modular, as is vector addition. Formally, we have the
following.
\begin{definition}
	\label{def:modular-op}
	An operator $\otimes:\Set{0,1}^s\times\Set{0,1}^s\to\Set{0,1}^s$  is
	called \textbf{modular} if there exists a partition
	$s=g_1+g_2+\cdots+g_K$, and  $K$ operators
	$\otimes_i:\Set{0,1}^{g_i}\times\Set{0,1}^{g_i}\to\Set{0,1}^{g_i}$
	such that for any $x,y\in\Set{0,1}^s$, $x\otimes y$ is equal to the
	concatenation $(x_1\otimes_1y_1)(x_2\otimes_2 y_2)\cdots 
	(x_K\otimes_K y_K)$ with $x=x_1 x_2 \cdots x_K$, $y=y_1 y_2 \cdots y_K$ and
	$|x_i|=|y_i|=g_i$ for every $i$.
	The \textbf{grain size
		of $\otimes$ in the given partition} is $\max\Set{g_i\mid 1\le i\le
		K}$, and the \textbf{grain size of $\otimes$} is the minimal grain
	size of $\otimes$ over all partitions.
	%\yehuda{Dont you want $\min$ instead of $\max$ in the grain def}\gal{no, if there is a grain of size $1$ and a grain of size $s-1$, the latter would be more dominant} \yehuda{it does not work with the way it is used in the next pages}.
\end{definition}
Note that any $s$-bits binary operator is trivially modular with grain
size at most $s$. However, small grain size facilitates parallelism
and pipelining by applying the operation on small parts of the operands
independently. Note also that the grain size depends on the way we
break down the operands; the best breakdown is the one that minimizes
the grain size.
%
% Modular operators allow for applying their sub-operators in a
% pipelined fashion. 
%In any case,
Given such a breakdown,
in case that all (cloud and local) links have bandwidth at least the grain size,
we can use pipelining to
convert the
logarithmic factor of \theoremref{thm-ccw-intervals-ub}
to an additive term, as the following theorem states.
\begin{theorem}\label{thm-aw-modular:appendix}
	% 	Let $Z_{\max} = {|\IR{j_{\max}}| + {s}/{\bLminR{j_\ell}} +
	% 		{s}/{\bC{\IR{j_c}}} }$, and
	Let $G = (V,E)$ be a graph of the wheel topology in the \CWC model.
	Suppose that $\otimes$ is modular with
	grain size $g$,
	and that $w(e) \ge g$ for every link $e\in E$.	
	Then \CCW can be solved in
	$O\left(Z_{\max}+\log n\right)$
	%	$O\left(Z_{\max}+|I_{j_{\max}}|\ceil{g\over\phi(I_{j_{\ell}})}+
	%	\ceil{g\over\bC{\IR{j_c}}}\log n\right)$
	rounds in the wheel settings.
\end{theorem}

Similarly to \corollaryref{cor-ub}, we can get get result for the uniform case.
\begin{corollary} \label{cor:modular-combining}
	In the uniform wheel topology with cloud bandwidth $\bc$ and local
	link bandwidth $\bl$ s.t. $\bl\ge\bc$, \CCW with an operation of
	grain size $g\le\bc$ can be executed in
	$O\left(\frac{s}{\bl}+\min\left(\sqrt{\frac{s}{\bc}},\frac{\bl}{\bc}\right)+\log n\right)$
	rounds.
	% 	\gal{shouldn't we prove it? or at least reference a similar corollary with similar arguments? where did the middle operand of the upper bound disappear?}
\end{corollary}
%\boaz{fill in differences from holistic}

\textbf{Proof of \theoremref{thm-aw-modular}:}
From a high level perspective,
modular combining is the same as holistic
combining, as presented in \theoremref{thm-ccw-intervals-ub} and \algref{alg:ccw-hi}.
%(\algref{alg:ccw-high:node} is
%slightly modified). % \yehuda{and 4?}.
All of the preprocessing steps remain unchanged.  The
difference is in the implementation of the low level steps
(\ref{ccw-startloop}--\ref{ccw-endloop}) and
the high level step (\ref{ccw-high}).

For a low level step, we note that the computation tree of \lemmaref{lem-lo}
is no longer
necessary; thanks to the {modularity} of operator $\otimes$, a simple
one-pass procedure suffices.  For interval $I=\interval{\ell}{r}$, the
algorithm forwards $S_\ell$ from node $\ell$ through the local links
all the way to node $r$, and every node along the way combines the
grains it receives with its local corresponding grain,
and forwards the result grain as soon as it is computed.
% relevant chunk \yehuda{you have not yet mentioned chunks or chunk size !} of its input before passing it on.

More formally, let $i\ne \ell$ be some node in $I$.  Let
$x=S_\ell^{i-1}$ be the operand that $i$ should receive from node
$i-1$, and let $y=S_i$. We consider the partition of $x$ and $y$
according to the grains of $\otimes$ as described in
\defref{def:modular-op}. %\yehuda{by the current definition $s$ is the
% size?!}\boaz{??}.
For every grain $x_j$ that $i$ fully receives, it
calculates locally the product $x_j \otimes_j y_j$ and proceeds to
send it immediately to node $i+1$.
\begin{lemma}\label{lem:pipe-lo}
	Let $\otimes$ be a modular operator with grain size $g$ as in
	\defref{def:modular-op},
	and assume that $w(e) \ge g$ for every link $e\in E$.
	Using pipelining, line \ref{ccw-local} of
	\algref{alg:ccw-hi} can be computed in an interval $I$ in
	$O\left({\frac{s}{\phi(I)}}+|I|\right)$
	%	$O\left({\frac{s}{\phi(I)}}+\ceil{ \frac{g}{\phi(I)} }\cdot|I|\right)$
	rounds.
\end{lemma}
\Proof
% The time to compute the first grain of the result, using pipelining,
% is $O(\ceil{g/\phi(I)}\cdot|I|)$. 
The number of messages required
to send all $s$ bits from a node $j$ to node $j+1$ using only local links is at least
$\ceil{s/\phi(I)}$. An intermediate node can compute the
result of a grain and start forwarding it to the next node after
%$\ceil{g/\phi(I)}$
$O(1)$
steps at most, since a complete grain is needed.
(either a grain was sent in its entirety, or a part of it was
and the rest can be sent in the next round.)
The lemma follows.
% Thus the
% overall time to compute all grains 
% is $O(|I|\cdot\ceil{g\over\phi(I)}+{s/\phi})$.
\QED
%\gal{I think we can get a tighter bound by summing over $\ceil{g/w(e)}$ for all local links $e$ in the interval}

\begin{corollary}\label{cor:pipe-lo}
	In the settings of \lemmaref{lem:pipe-lo},
	line \ref{ccw-local} of
	\algref{alg:ccw-hi} can be computed in
	$O\left({\frac{s}{\phi(I_{j_\ell})}}+|I_{j_{\max}}|\right) \le O(\Zmax)$
	rounds.
\end{corollary}

\bigskip
The pipelining strategy applies also to the tree nodes computed
in line \ref{ccw-high} of \algref{alg:ccw-hi}. Specifically, we need to
change \algref{alg:ccw-high:node} to work grain-by-grain.
%as follows.
Note that we assume the constant-factor multiplexing of
Step \ref{ccw-1} of \algref{alg:ccw-hi}, and thus describe the algorithm
as if all intervals are operating in complete parallelism.
In addition, we assume the bandwidth of all links to be a multiple of $g$
(note that this assumption may only incur a constant factor slowdown,
as a link $e$ passing a message of size $w(e)$ can be simulated
with $2$ rounds of passing messages of sizes
$\floor{w(e)/g}\cdot g$ and $(w(e) \bmod g)$ since $w(e) \ge g$).

Suppose that interval $I$ is
in charge of filling in the value of a tree node $y$ with children
$y_\ell$ and $y_r$.
We assume that the order of reading and writing a string $S$ in \CR
and \CW is sequential, i.e., the first bits of $S$ are retrieved (or
written, resp.) first. We run, in parallel, \CR on $y_\ell$ and $y_r$,
and we also run \CW of $y$ in
parallel to them. We can implement this parallelization using multiplexing of the nodes of $I$,
while maintaining the same round complexity:
%at the cost of a
%constant factor slowdown: each node is taking part of only a constant number of
%\CR and \CW actions concurrently.
the same operations that make up the \CR and \CW actions would still occur,
it is just the order of the schedule that is tweaked.
%\gal{previously it said that there's a constant factor slowdown}
%\yehuda{not clear. I did not understand}. 
As soon as a grain of $y_\ell$ and the corresponding grain of
$y_r$ are available, the node of $I$ that read them from the cloud
computes the corresponding grain of the result and writes it using
$\CW$. This way, computing a grain at a tree-node requires
%$O(\ceil{g/\bc(I)|})$
$O(1)$ rounds.
%\gal{I think this is wrong. oof.}
Hence the first grain is computed at the
root after
%$O(\ceil{g/\bc(I)}\log n)$
$O(\log n)$ rounds.
\CW requires $O(\Zmax)$ rounds, 
%In every round we can
%send $\min(\bc(I),\phi(I))$ bits,
and hence the last grain is written
$O(Z_{\max})$ rounds later.
%\yehuda{not clear enough.  how do we know
%the pipelining stages do not interfere
%with each other on different links?}
Thus we obtain the following result.
\begin{lemma}\label{lem:pipe-hi}
	Let $\otimes$ be a modular operator with grain size $g$ as in
	\defref{def:modular-op},
	and assume that $w(e) \ge g$ for every link $e\in E$.
	Using pipelining, line \ref{ccw-high} of
	\algref{alg:ccw-hi} can be computed in 
	$O\left(Z_{\max}+\log n\right)$
	%	$O\left(Z_{\max}+\ceil{g\over\bc(I_{j_c})}\log n\right)$
	rounds.
\end{lemma}


\theoremref{thm-aw-modular} follows from \corollaryref{cor:pipe-lo} and
\lemmaref{lem:pipe-hi}.















%%% Local Variables:
%%% mode: latex
%%% TeX-master: "cwc"
%%% End:
